# Supplementary material for: 3-coloring triangle-free planar graphs with a precolored 9-cycle
Source: arXiv:1709.09428 ancillary file (2017-09-27)

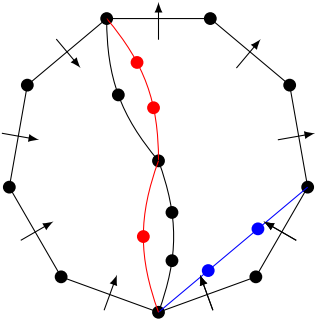



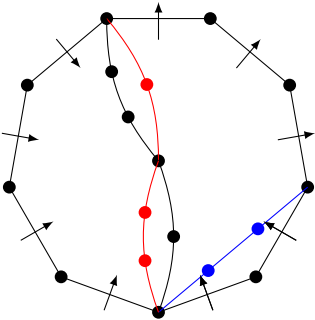



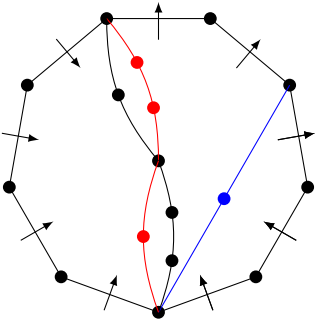



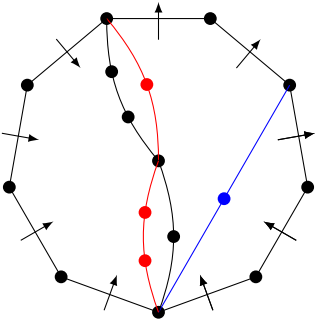

Supplement: Supplementary file 2 [file bernard_555_BBB_2.tikz.pdf]
