# Supplementary material for: 3-coloring triangle-free planar graphs with a precolored 9-cycle
Source: arXiv:1709.09428 ancillary file (2017-09-27)

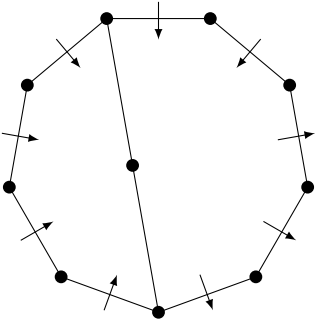

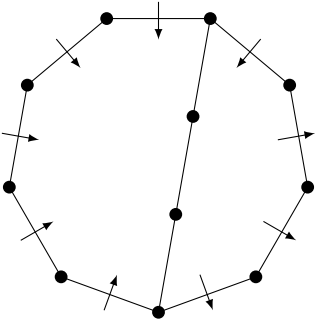

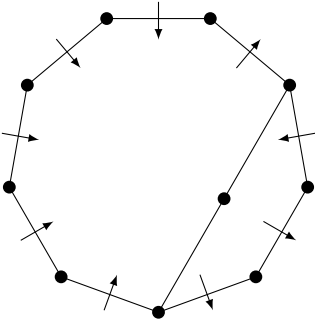

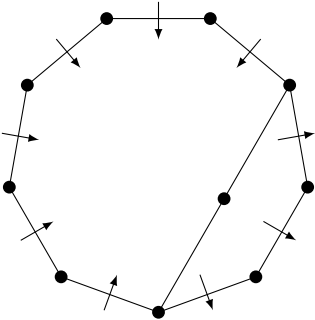

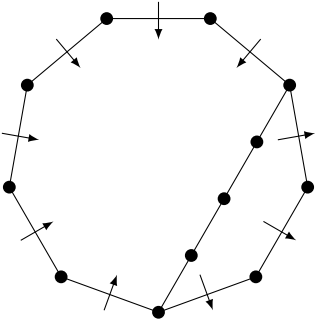

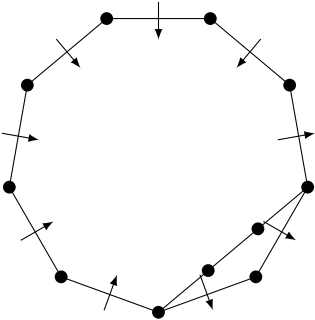

Supplement: Supplementary file 6 [file bernard_5_alone.tikz.pdf]
